# Supplementary material for: Exploring Event Camera-based Odometry for Planetary Robots
Source: arXiv:2204.05880 source file (2022-07-29)
Supplement: Supplementary file 1 [file supplementary.tex]

\clearpage

\section{Supplementary material}

\Cref{tab:evaluation-sequences} lists all the sequences and datasets used for evaluation.

% Please add the following required packages to your document preamble:
% \usepackage{booktabs}
% \usepackage{multirow}
\begin{table*}[t]
\centering
\begin{tabular}{@{}llcc@{}}
\toprule
Dataset                                                                                                                                   & \multicolumn{1}{c}{Sequence} & Trajectory length {[}m{]} & Sensing modalities                                                                                                                         \\ \midrule
\multirow{5}{*}{\begin{tabular}[c]{@{}l@{}}Simulated MARS\\ environment\\ on real drone flight\\ trajectories\end{tabular}}               & Mars Straight                & tbd                       & \multirow{5}{*}{\begin{tabular}[c]{@{}c@{}}Simulated Davis346:\\ grayscale frames,\\ events, IMU; pose GT,\\ depthmap GT\end{tabular}} \\
                                                                                                                                          & Mars Circle                  & tbd                       &                                                                                                                                            \\
                                                                                                                                          & Mars Eight                   & tbd                       &                                                                                                                                            \\
                                                                                                                                          & Mars Vertical Circle         & tbd   &                                                                                                                                            \\
                                                                                                                                          & Mars Mellon                  & tbd                       &                                                                                                                                            \\ \midrule
\multirow{14}{*}{\begin{tabular}[c]{@{}l@{}}Event-Camera Dataset~\cite{Mueggler17ijrr}\\ (real data in \\ office environment\\ with artificial texture)\end{tabular}} & Boxes 6DOF                   & 69.9                      & \multirow{14}{*}{\begin{tabular}[c]{@{}c@{}}DAVIS 240:\\ grayscale frames,\\ events,\\ IMU;\\ Optitrack GT\end{tabular}}                   \\
                                                                                                                                          & Boxes Translation            & 65.2                      &                                                                                                                                            \\
                                                                                                                                          & Dynamic 6DOF                 & 39.6                      &                                                                                                                                            \\
                                                                                                                                          & Dynamic Translation          & 30.1                      &                                                                                                                                            \\
                                                                                                                                          & HDR Boxes                    & 55.1                      &                                                                                                                                            \\
                                                                                                                                          & HDR Poster                   & 55.4                      &                                                                                                                                            \\
                                                                                                                                          & Poster 6DOF                  & 61.1                      &                                                                                                                                            \\
                                                                                                                                          & Poster Translation           & 49.3                      &                                                                                                                                            \\
                                                                                                                                          & Shapes 6DOF                  & 47.6                      &                                                                                                                                            \\
                                                                                                                                          & Shapes Translation           & 56.1                      &                                                                                                                                            \\ \cmidrule(lr){2-3}
                                                                                                                                          & Boxes Rotation               & 14.9                      &                                                                                                                                            \\
                                                                                                                                          & Dynamic Rotation             & 10.5                      &                                                                                                                                            \\
                                                                                                                                          & Shapes Rotation              & 15.7                      &                                                                                                                                            \\
                                                                                                                                          & Poster Rotation              & 16.9                      &                                                                                                                                            \\ \bottomrule
\end{tabular}
\caption{Evaluation sequences}
\label{tab:evaluation-sequences}
\end{table*}
